# Supplementary material for: Electronic structure and phase stability of oxide semiconductors: Performance of dielectric-dependent hybrid functional DFT, benchmarked against $GW$ band structure calculations and experiments
Source: arXiv:1508.02174 source file (2015-08-11)
Supplement: Supplementary file 1 [file Supplemental_Material.pdf]

# Supplemental Material for:
# "Electronic structure and phase stability of oxide semiconductors: performance of dielectric-dependent hybrid functional DFT, benchmarked against $GW$ bandstructure calculations and experiments"


Matteo Gerosa

*Department of Energy, Politecnico di Milano, via Ponzio 34/3, 20133 Milano, Italy*

Carlo Enrico Bottani

*Department of Energy, Politecnico di Milano, via Ponzio 34/3, 20133 Milano, Italy and Center for Nano Science and Technology @Polimi, Istituto Italiano di Tecnologia, via Pascoli 70/3, 20133 Milano, Italy*

Lucia Caramella and Giovanni Onida

*Dipartimento di Fisica, Università degli Studi di Milano, Milano, Italy and European Theoretical Spectroscopy Facility (ETSF)*

Cristiana Di Valentin and Gianfranco Pacchioni

*Dipartimento di Scienza dei Materiali, Università di Milano-Bicocca, via R. Cozzi 53, 20125 Milan, Italy*



(Dated: January 27, 2015)


## I. HYBRID DFT AND $GW$: COMPUTATIONAL DETAILS

As discussed in the main text, DFT hybrid functional calculations can be very expensive using a plane-waves (PW) basis set. In particular, the computational effort strongly depends on the choice of the Brillouin-zone (BZ) sampling. This is illustrated in Fig. S1 for the test case of MgO.

In Table S1 we report $k$- and $q$-point grids of our PW calculations performed with the QUANTUM ESPRESSO package. In total energy calculations using the CRYSTAL09 code, convergence studies on the BZ sampling were carried out so as to ensure accuracy within 1 meV on total energies for the various phases. This corresponds to 10x10x10 for MgO, and at least 14x14x14 for ZnO, 6x6x6 for $TiO_2$, 6x6x6 for $ZrO_2$, and 4x4x4 for $WO_3$.

Table S2 collects various cutoff parameters entering $GW$ calculations for the materials investigated in Section III A of the main text. The meaning of the single cutoff parameters is discussed in Section II C of the main text.

TABLE S1: Computational parameters of DFT PW calculations: $k$- and $q$-point BZ sampling and PW kinetic energy cutoff $E_{\rm cut}$ (in Ry).

| | $k$-point grid | $q$-point grid | $E_{\rm cut}$ |
|---|---|---|---|
| MgO | 4x4x4 | 4x4x4 | 500 |
| ZnO | 4x4x2 | 4x4x2 | 300 |
| $TiO_2$ | 4x4x2 | 4x4x2 | 150 |
| $ZrO_2$ | 4x4x4 | 4x4x4 | 120 |
| $WO_3$ | 2x2x2 | 2x2x2 | 100 |

TABLE S2: Computational cutoff parameters used in $GW$ calculations: cutoff energies $E^{\rm eps}_{\rm cut}$ and $E^{\rm xc}_{\rm cut}$ (in Ry) controlling the size of the dielectric matrix in reciprocal space and the number of plane waves in the expansion of xc potential, respectively; number of empty states included in the evaluation of the polarizability $\chi$ and of the Coulomb hole (CH) term.

| | | | Empty states | |
|---|---|---|---|---|
| | $E^{\rm eps}_{\rm cut}$ | $E^{\rm xc}_{\rm cut}$ | $\chi$ | $\Sigma_{\rm CH}$ |
| MgO | 90 | 80 | 300 | 900 |
| ZnO | 70 | 200 | 200 | 2750 |
| $TiO_2$ | 14 | 50 | 500 | 1300 |
| $ZrO_2$ | 25 | 50 | 500 | 2100 |
| $WO_3$ | 16 | 60 | 800 | 2300 |

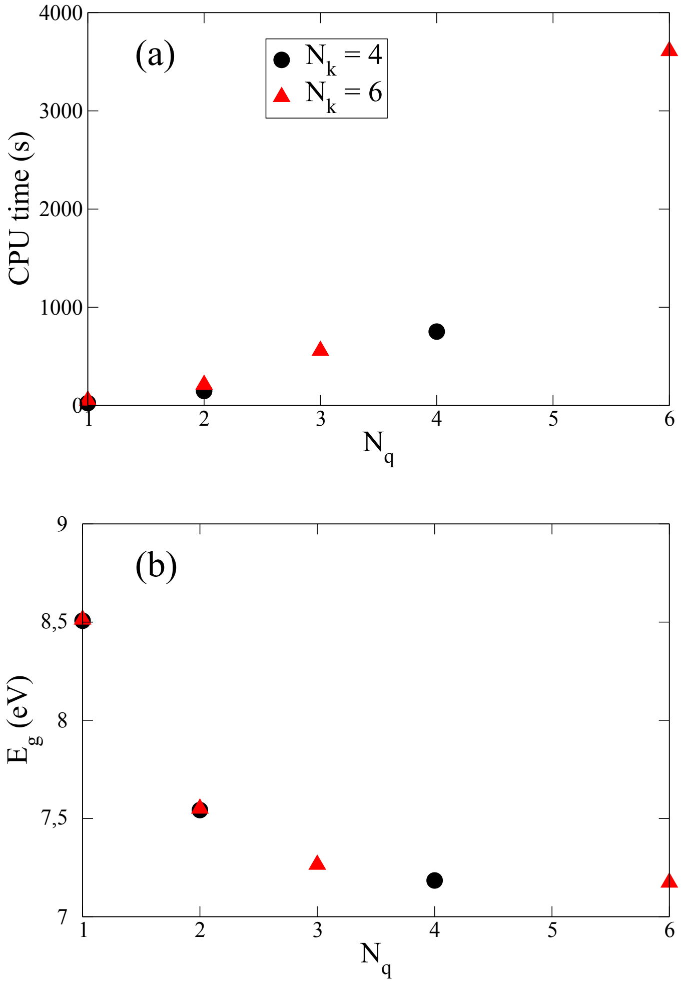


FIG. S1: (a) CPU time and (b) band gap of MgO in hybrid PBE0 calculations with QUANTUM ESPRESSO, using $k$- and $q$-point grids of different sizes; $N_k$ and $N_q$ indicate, respectively, $N_k \times N_k \times N_k$ and $N_q \times N_q \times N_q$ Monkhorst-Pack grids.

## II. LATTICE PARAMETERS

In Table S3 we report experimental lattice constants used in all the relevant calculations presented in the main text (see Section III A), together with the results of the geometry optimizations performed within LDA and PBE with QUANTUM ESPRESSO for the purpose of validating pseudopotentials. The tendency of LDA and GGA to underestimate and overestimate, respectively, lattice constants is confirmed by our calculations.

Results of geometry optimizations carried out with CRYSTAL09 for the phases not included in Table VII of the main text are reported in Table S4. Calculations were carried out within PBE, PBE0 and dielectric-dependent PBE0, PBE0$\alpha^{(1)}_{\text{PBE}}$.

TABLE S3: Lattice constants computed within LDA and PBE with QUANTUM ESPRESSO, and comparison with experiments.

| | Type | Parameter | LDA | PBE | Expt.[a] |
|---|---|---|---|---|---|
| MgO | rocksalt | a (Å) | 4.156 | 4.230 | 4.212 |
| ZnO | wurtzite | $a$ (Å) | 3.172 | 3.242 | 3.249 |
| | | $c$ (Å) | 5.113 | 5.215 | 5.207 |
| | | $u$ | 0.379 | 0.380 | 0.382 |
| $TiO_2$ | anatase | $a$ (Å) | 3.748 | 3.795 | 3.781 |
| | | $c$ (Å) | 9.427 | 9.645 | 9.515 |
| | | $u$ | 0.209 | 0.207 | 0.208 |
| $ZrO_2$ | tetragonal | $a$ (Å) | 3.559 | 3.613 | 3.571 |
| | | $c$ (Å) | 5.116 | 5.268 | 5.182 |
| | | $d_z$ | 0.0434 | 0.0566 | 0.0574 |
| $WO_3$ | $\gamma$-monoclinic | $a$ (Å) | 7.325 | 7.437 | 7.306 |
| | | $b$ (Å) | 7.477 | 7.683 | 7.540 |
| | | $c$ (Å) | 7.557 | 7.777 | 7.692 |
| | | $\beta$ (°) | 90.98 | 90.10 | 90.88 |

[a]Experimental lattice constants are found in the following references: Ref. 1 for MgO, Ref. 2 for ZnO, Ref. 3 for $TiO_2$, Ref. 4 for $ZrO_2$, Ref. 5 for $WO_3$.

TABLE S4: Optimized cell parameters for selected polymorphs of the studied materials, computed at different levels of theory with CRYSTAL09.

| | Type | Parameter | PBE | PBE0 | PBE0$\alpha^{(1)}_{\mathrm{PBE}}$ | Expt.[a] |
|---|---|---|---|---|---|---|
| ZnO | zinc-blende | a (Å) | 4.584 | 4.547 | 4.541 | 4.620 |
| $TiO_2$ | rutile | a (Å) | 4.621 | 4.568 | 4.588 | 4.587 |
| | | c (Å) | 3.002 | 2.978 | 2.987 | 2.954 |
| | brookite | a (Å) | 9.260 | 9.177 | 9.201 | 9.174 |
| | | b (Å) | 5.518 | 5.441 | 5.464 | 5.449 |
| | | c (Å) | 5.215 | 5.156 | 5.176 | 5.138 |
| $ZrO_2$ | cubic | a (Å) | 5.148 | 5.103 | 5.112 | 5.110 |
| | monoclinic | a (Å) | 5.224 | 5.189 | 5.192 | 5.151 |
| | | b (Å) | 5.293 | 5.246 | 5.253 | 5.212 |
| | | c (Å) | 5.382 | 5.330 | 5.334 | 5.317 |
| | | $\beta$ (°) | 99.57 | 99.51 | 99.51 | 99.23 |
| $WO_3$ | cubic | a (Å) | 3.834 | 3.786 | 3.811 | 3.772 |
| | tetragonal | a (Å) | 5.345 | 5.281 | 5.295 | 5.250 |
| | | c (Å) | 4.058 | 4.018 | 4.031 | 3.915 |
| | $\varepsilon$-monoclinic | a (Å) | 5.532 | 5.286 | 5.295 | 5.277 |
| | | b (Å) | 5.259 | 5.193 | 5.202 | 5.155 |
| | | c (Å) | 7.880 | 7.794 | 7.805 | 7.663 |
| | | $\beta$ (°) | 91.16 | 91.18 | 91.19 | 91.76 |
| | triclinic | a (Å) | 7.430 | 7.334 | 7.343 | 7.313 |
| | | b (Å) | 7.658 | 7.592 | 7.619 | 7.525 |
| | | c (Å) | 7.854 | 7.781 | 7.799 | 7.689 |
| | | $\alpha$ (°) | 89.21 | 89.23 | 89.28 | 88.85 |
| | | $\beta$ (°) | 90.61 | 90.55 | 90.52 | 90.91 |
| | | $\gamma$ (°) | 90.72 | 90.64 | 90.60 | 90.94 |
| | orthorombic | a (Å) | 7.518 | 7.419 | 7.430 | 7.341 |
| | | b (Å) | 7.779 | 7.705 | 7.715 | 7.570 |
| | | c (Å) | 7.926 | 7.848 | 7.859 | 7.754 |

[a]Experimental lattice constants are found in the following references: Ref. 6 for zinc-blende ZnO; Refs. 7,8 for rutile and brookite $TiO_2$; Refs. 9,10 for cubic and monoclinic $ZrO_2$; Refs. 11–15 for cubic, tetragonal, low-temperature $\varepsilon$-monoclinic. triclinic and orthorombic $WO_3$.

[1] D. R. Lide (CRC Press/Taylor and Francis, Boca Raton, FL, 1998/1999), 79th ed.

[2] D. F. Croxall, R. C. C. Ward, C. A. Wallace, and R. C. Kell, J. Cryst. Growth **22**, 117 (1974).

[3] M. Horn, C. F. Schwerdtfeger, and E. P. Meagher, Z. Kristallogr. **136**, 273 (1972).

[4] E. V. Stefanovich, A. L. Shluger, and C. R. A. Catlow, Phys. Rev. B **49**, 11560 (1994).

[5] B. O. Loopstra and H. M. Rietveld, Acta Crystallogr., Sect. B **25**, 1420 (1969).

[6] W. H. Bragg and J. A. Darbyshire, J. Met. **6**, 238 (1954).

[7] R. J. Swope, J. R. Smyth, and A. C. Larson, Am. Mineral. **80**, 448 (1995).

[8] E. P. Meagher and G. A. Lager, Can. Mineral. **17**, 77 (1979).

[9] R. P. Ingel and D. Lewis, J. Am. Ceram. Soc. **69**, 325 (1986).

[10] C. J. Howard, R. J. Hill, and B. E. Reichert, Acta Crystallogr., Sect. B **44**, 116 (1988).

[11] W. A. Crichton, P. Bouvier, and A. Grzechnik, Mater. Res. Bull. **38**, 289 (2003).

[12] W. L. Kehl, R. G. Hay, and D. Wahl, J. Appl. Phys. **23**, 212 (1952).

[13] E. K. H. Salje, S. Rehmann, F. Pobell, D. Morris, K. S. Knight, T. Herrmannsdörfer, and M. T. Dove, J. Phys.: Condens. Matter **9**, 6564 (1997).

[14] P. M. Woodward, A. W. Sleight, and T. Vogt, J. Phys. Chem. Solids **56**, 1255 (1995).

[15] E. Salje, Acta Crystallogr., Sect. B **33**, 574 (1977).
